# Supplementary material for: IELM: An Open Information Extraction Benchmark for Pre-Trained Language Models
Source: arXiv:2210.14128 source file (2022-10-25)
Supplement: Supplementary file 3 [file unmapped_bertlarge_kbp.tex]

SF13\_ENG\_001 & Bashardost was born in 1965 in the southern Ghanzi province and his family migrated to Iran and then to Pakistan after successive coup and factional fighting in Afghanistan . & (Bashardost, in, The Southern Ghanzi Province) $\rightarrow$ (Ramazan Bashardost, per:stateorprovince\_of\_birth, The Southern Ghanzi Province)\\ \hline
SF13\_ENG\_012 & Gadahn , also known as Azzam the American , was born in 1978 . & (Gadahn, ,, Azzam) $\rightarrow$ (Adam Gadahn, per:alternate\_names, Azzam)\\ \hline
SF13\_ENG\_015 & Besides her sister , Philip , survivors include a son , Graham ; three daughters , Sidney , Gillian and Alexia ; and three grandchildren . & (Her Sister, ,, Philip) $\rightarrow$ (Lucille Clifton, per:siblings, Philip)\\ \hline
SF13\_ENG\_015 & The poet laureate of Maryland from 1979 to 1985 , Clifton was a writer in residence at Coppin State College , now Coppin State University , a historically black college in Baltimore . & (Clifton, in, Coppin State College) $\rightarrow$ (Lucille Clifton, per:school\_attended, Coppin State College)\\ \hline
SF13\_ENG\_015 & Her father , Samuel , was a steelworker ; her mother , Thelma , worked in a laundry . & (Her Father, ,, Samuel) $\rightarrow$ (Lucille Clifton, per:parents, Samuel)\\ \hline
SF13\_ENG\_015 & Lucille Clifton , a distinguished American poet whose work trained lenses wide and narrow on the experience of being black and female in the 20th century , exploring vast subjects like the indignities of history and intimate ones like the indignities of the body , died on Saturday in Baltimore . & (Lucille Clifton, ,, poet) $\rightarrow$ (Lucille Clifton, per:title, poet)\\ \hline
SF13\_ENG\_015 & The precise cause of death had not been determined , her sister , Elaine Philip , told The Associated Press on Sunday . & (Her Sister, ,, Elaine Philip) $\rightarrow$ (Lucille Clifton, per:siblings, Elaine Philip)\\ \hline
SF13\_ENG\_037 & CLAUDE CHABROL , PIONEER FRENCH FILMMAKER , DIES AT 80 Joseph Berger contributed reporting from New York , and Maia de la Baume contributed from Paris . & (Claude Chabrol, ,, Pioneer French Filmmaker) $\rightarrow$ (Claude Chabrol, per:title, Pioneer French Filmmaker)\\ \hline
SF13\_ENG\_037 & Chabrol ' s survivors also include his third wife , Aurore Pajot , who acted as his script supervisor on nearly all of his movies from 1968 on and whom he married in 1981 ; and Pajot ' s daughter , Cecile Maistre , who was an assistant director on his films and wrote the script with him for " The Girl Cut in Two " ( 2007 ) . & (His Third Wife, ,, Aurore Pajot) $\rightarrow$ (Claude Chabrol, per:spouse, Aurore Pajot)\\ \hline
SF13\_ENG\_044 & Dominick Dunne , a novelist and journalist who chronicled true - crime tales of the rich and infamous , including O . J . Simpson and Claus von Bulow , and in turn became a celebrity in his own right , died of bladder cancer Aug . 26 at his home in New York City . & (Dominick Dunne, ,, A Novelist) $\rightarrow$ (Dominick Dunne, per:title, A Novelist)\\ \hline
SF13\_ENG\_044 & Dunne and his wife , Ellen Griffin Dunne , known as Lenny , were married in 1954 . & (His Wife, ,, Ellen Griffin Dunne) $\rightarrow$ (Dominick Dunne, per:spouse, Ellen Griffin Dunne)\\ \hline
SF13\_ENG\_044 & Dunne was born in 1925 in Hartford , Connecticut , to a wealthy Roman Catholic family and grew up in some of the same social circles as the Kennedys . & (Dunne, ,, Connecticut) $\rightarrow$ (Dominick Dunne, per:stateorprovince\_of\_birth, Connecticut)\\ \hline
SF13\_ENG\_049 & A professor emeritus at Yale University , Mandelbrot was born in Poland but as a child moved with his family to France where he was educated . & (Mandelbrot, ,, Yale University) $\rightarrow$ (Benoit Mandelbrot, per:employee\_or\_member\_of, Yale University)\\ \hline
SF13\_ENG\_058 & Access Industries , a privately held company founded in 1986 by Len Blavatnik , has a diverse portfolio of investments in industry , real estate , media and telecommunications . & (Access Industries, ,, A Privately Held Company) $\rightarrow$ (Access Industries, properties, A Privately Held Company)\\ \hline
SF13\_ENG\_079 & Water and its links to development , peace and conflict were key words in the annual sessions , Anders Berntell , executive director of Stockholm International Water Institute ( SIWI ) , said in his opening address . & (Stockholm International, ,, Anders Berntell) $\rightarrow$ (Stockholm International Water Institute, per:top\_members\_or\_employees, Anders Berntell)\\
