# Supplementary material for: IELM: An Open Information Extraction Benchmark for Pre-Trained Language Models
Source: arXiv:2210.14128 source file (2022-10-25)
Supplement: Supplementary file 4 [file unmapped_bertlarge_wikidata.tex]

Nick\_Aldis & He was also a co - presenter of " Britain ' s Strongest Man " on Challenge TV in the United Kingdom . & (Challenge Tv, in, The United Kingdom) $\rightarrow$ (Challenge TV, in, united\_kingdom.Q145)\\ \hline
Douglas\_Bader & At the age of two , Bader joined his parents in India for a year . & (His Parents, in, India) $\rightarrow$ (douglas\_bader.Q348780, in, india.Q668)\\ \hline
Douglas\_Bader & He remained in France after the war , where , having attained the rank of major , he died in 1922 of complications from those wounds in a hospital in Saint - Omer , the same area where Bader would bail out and be captured in 1941 . & (He, in, France) $\rightarrow$ (douglas\_bader.Q348780, in, france.Q142)\\ \hline
Douglas\_Bader & On 2 July 1941 he was awarded the bar to his DSO. & (He, was awarded the bar, his DSO) $\rightarrow$ (douglas\_bader.Q348780, was awarded the bar, distinguished\_service\_order.Q615838) \\ \hline
Helen\_Storrow & His father , also named James Jackson Storrow , was a prominent attorney , whose clients included Alexander Graham Bell and the government of Venezuela ; his mother , Ann Maria Perry , was the grandchild of naval hero Commodore Oliver Hazard Perry , and a distant cousin of President Thomas Jefferson . & (His Father, was, A Prominent Attorney) $\rightarrow$ (His Father, occupation.P106, lawyer.Q40348)\\ \hline
Helen\_Storrow & Helen Storrow Helen Osborne Storrow was a prominent American philanthropist , early Girl Scout leader , and chair of the World Committee of the World Association of Girl Guides and Girl Scouts for eight years . & (Helen Osborne Storrow, was, A Prominent American Philanthropist) $\rightarrow$ (helen\_storrow.Q5703224, place\_of\_birth.P19, united\_states.Q30)\\ \hline
Jacob\_Van\_Ruisdael & His cousin Jacob was a registered Mennonite in Amsterdam . & (His Cousin, was, A Registered Mennonite) $\rightarrow$ (His Cousin, was, A Registered Mennonite)\\ \hline
Jacob\_Van\_Ruisdael & He appears to have been strongly influenced by other contemporary local Haarlem landscapists , most notably Cornelis Vroom and Allaert van Everdingen . & (He, have been strongly influenced by, landscape painting) $\rightarrow$ (jacob\_van\_ruisdael.Q213612, have been strongly influenced by, landscape\_art.Q191163)\\ \hline
Liaquat\_Ali\_Khan & Liaquat Ali Khan was educated at the Aligarh Muslim University in India , and then at Oxford University in the United Kingdom . & (Liaquat Ali Khan, in, India) $\rightarrow$ (liaquat\_ali\_khan.Q295713, in, india.Q668)\\ \hline
Pauline\_Baynes & Baynes began her education at a convent school . & (Her Education, at, A Convent School) $\rightarrow$ (pauline\_baynes.Q101951, at, catholic\_school.Q1138671)\\ \hline
Pauline\_Baynes & Her most vivid recollection of their New Year ' s Eve lunch at Magdalen College was of his gleefully picking nuts out of a bowl of Brussels sprouts . & (Their New Year'S Eve Lunch, at, Magdalen College) $\rightarrow$ (pauline\_baynes.Q101951, at, magdalen\_college,\_oxford.Q81162)\\ \hline
Pauline\_Baynes & By the time that she left , she had already formed the ambition of becoming an illustrator . & (She, formed the ambition of becoming, An Illustrator) $\rightarrow$ (pauline\_baynes.Q101951, formed the ambition of becoming, illustrator.Q644687)\\ \hline
Thor\_Heyerdahl & He was an atheist . & (He, was, An Atheist) $\rightarrow$ (thor\_heyerdahl.Q133622, was, An Atheist)\\ \hline
Thor\_Heyerdahl & He is buried in the garden of the family home in Colla Micheri . & (He, is buried, Colla Micheri) $\rightarrow$ (thor\_heyerdahl.Q133622, is buried, colla\_micheri.Q3647771)\\ \hline
Neville\_Southall & He moved on to Cheshire County League club Winsford United at the age of 20 . & (He, to, Cheshire County League Club Winsford United) $\rightarrow$ (neville\_southall.Q436650, to, winsford\_united\_f.c..Q5213266)\\ \hline
Neville\_Southall & He later became a player - coach at York City , Rhyl , Shrewsbury Town and Dagenham \& Redbridge . & (He, became, A Player-Coach) $\rightarrow$ (neville\_southall.Q436650, occupation.P106, A Player-Coach)\\ \hline
John\_Maynard\_Keynes & After the war , Winston Churchill attempted to check the rise of Keynesian policy - making in the United Kingdom and used rhetoric critical of the mixed economy in his 1945 election campaign . & (Keynesian Policy-Making, in, The United Kingdom) $\rightarrow$ (john\_maynard\_keynes.Q9317, in, united\_kingdom.P145)\\ \hline
John\_Maynard\_Keynes & Apart from Great Britain , Keynes ' s attention was primarily focused on the United States . & (Keynes'S Attention, was, The United States) $\rightarrow$ (john\_maynard\_keynes.Q9317, was, united\_states.Q30)\\ \hline
John\_Maynard\_Keynes & John Maynard Keynes John Maynard Keynes , 1st Baron Keynes , was a British economist , whose ideas fundamentally changed the theory and practice of macroeconomics and the economic policies of governments . & (John Maynard Keynes, was, A British Economist) $\rightarrow$ (john\_maynard\_keynes.Q9317, was, united\_kingdom.P145)\\ \hline
Ernst\_Haeckel & Ernst Haeckel Ernst Heinrich Philipp August Haeckel was a German zoologist , naturalist , philosopher , physician , professor , marine biologist , and artist who discovered , described and named thousands of new species , mapped a genealogical tree relating all life forms , and coined many terms in biology , including " ecology " , " phylum " , " phylogeny " , and " Protista . " & (August Haeckel, was, A German Zoologist) $\rightarrow$ (ernst\_haeckel.Q48246, was, germany.Q183)\\ \hline
Ernst\_Haeckel & Haeckel was awarded the title of Excellency by Kaiser Wilhelm II in 1907 and the Linnean Society of London ' s prestigious Darwin - Wallace Medal in 1908 . & (Haeckel, was awarded the, Excellency) $\rightarrow$ (ernst\_haeckel.Q48246, award\_received.P166, Excellency)\\ \hline
Ernst\_Haeckel & He was also a pacifist until the First World War , when he wrote propaganda in favor of the war . & (He, was, A Pacifist) $\rightarrow$ (ernst\_haeckel.Q48246, was, A Pacifist)\\
