# Supplementary material for: IELM: An Open Information Extraction Benchmark for Pre-Trained Language Models
Source: arXiv:2210.14128 source file (2022-10-25)
Supplement: Supplementary file 5 [file unmapped_gpt2xl_kbp.tex]

SF13\_ENG\_009 & He took office in 2006 by defeating longtime incumbent Anwar Chowdhry from Pakistan, who was later barred for alleged financial corruption. & (Longtime Incumbent Anwar Chowdhry, from, Pakistan) $\rightarrow$ (Anwar Chowdhry, per:countries\_of\_residence, Pakistan)\\ \hline
SF13\_ENG\_012 &  The message also featured several appearances of Adam Gadahn, also known as Azzam al-Amriki, an American who grew up in Riverside County and converted to Islam and joined al-Qaida. & (Adam Gadahn, also, Azzam Al-Amriki) $\rightarrow$ (Adam Gadahn, per:alternate\_names, Azzam Al-Amriki); (Adam Gadahn, ,, Azzam Al-Amriki) $\rightarrow$ (Adam Gadahn, ,, Azzam Al-Amriki)\\ \hline
SF13\_ENG\_014 &  Mohammed Oudeh, a former math teacher who became the mastermind of the deadly attack on Israeli athletes at the 1972 Munich Olympics, died Friday in Damascus. & (Mohammed Oudeh, ,, teacher) $\rightarrow$ (Mohammed Oudeh, per:title, teacher)\\ \hline
SF13\_ENG\_014 &  He settled in the West Bank town of Ramallah, but in 1999, after a trip to Jordan, he was barred by Israel from returning. & (He, in, The West Bank Town) $\rightarrow$ (Mohammed Oudeh, per:cities\_of\_residence, The West Bank Town)\\ \hline
SF13\_ENG\_014 &  Mohammed Oudeh, a former math teacher who became the mastermind of the deadly attack on Israeli athletes at the 1972 Munich Olympics, died Friday in Damascus. & (Mohammed Oudeh, ,, A Former Math Teacher) $\rightarrow$ (Mohammed Oudeh, per:title, A Former Math Teacher)\\ \hline
SF13\_ENG\_014 &  In later years, as a graying member of the Palestinian old guard, Oudeh, most commonly known by his guerrilla name, Abu Daoud, showed no remorse for the botched hostage taking and killings of 11 members of the Israeli Olympic team that shook the world. & (Oudeh, ,, Abu Daoud) $\rightarrow$ (Mohammed Oudeh, per:alternate\_names, Abu Daoud)\\ \hline
SF13\_ENG\_015 &  After her husband died in 1984, Clifton taught at the University of California at Santa Cruz before returning to Maryland in 1989. & (Clifton, of, Santa Cruz) $\rightarrow$ (Lucille Clifton, per:cities\_of\_residence, Santa Cruz)\\ \hline
SF13\_ENG\_015 &  Lucille Clifton, a National Book Award-winning poet and Pulitzer finalist, has died. & (Lucille Clifton, ,, poet) $\rightarrow$ (Lucille Clifton, per:title, poet)\\ \hline
SF13\_ENG\_015 &  When she was a girl, Lucille Clifton sat on her mother's lap and listened to her recite poetry. & (Lucille Clifton, ,, A Girl) $\rightarrow$ (Lucille Clifton, gender, A Girl)\\ \hline
SF13\_ENG\_015 &  In 1967, they moved to Baltimore, and Clifton worked in Washington for the old U.S. Office of Education. & (They, to, Baltimore) $\rightarrow$ (Lucille Clifton, per:cities\_of\_residence, Baltimore)\\ \hline
SF13\_ENG\_015 &  Clifton's sister, Elaine Philip, said the former poet laureate of Maryland passed away Saturday morning at Johns Hopkins University Hospital in Baltimore. & (Clifton'S Sister, ,, Elaine Philip) $\rightarrow$ (Lucille Clifton, per:siblings, Elaine Philip)\\ \hline
SF13\_ENG\_018 &  Harvey Pekar, the writer of comics whose autobiographical comic book series "American Splendor" chronicled his life as a filing clerk, record collector, freelance jazz critic and one of life's all-around misfits, was found dead July 12 at his home near Cleveland. & (Harvey Pekar, ,, writer) $\rightarrow$ (Harvey Pekar, per:title, writer)\\ \hline
SF13\_ENG\_018 &  Pekar attended what became Case Western Reserve University, served in the Navy in the late 1950s and worked a series of menial jobs before taking a 30-year jobas a filing clerk at a VA hospital in Cleveland. & (Pekar, what became, Case Western Reserve University) $\rightarrow$ (Harvey Pekar, per:schools\_attended, Case Western Reserve University)\\ \hline
SF13\_ENG\_025 &  Kissel, 46, of Adrian, Michigan, was convicted of drugging then bashing her husband Robert to death in a luxury Hong Kong apartment and sentenced to life in prison in September 2005. & (Kissel, ,, Adrian) $\rightarrow$ (Nancy Kissel, per:cities\_of\_residence, Adrian); (Kissel, ,, Michigan) $\rightarrow$ (Nancy Kissel, per:statesorprovinces\_of\_residence, Michigan)\\ \hline
SF13\_ENG\_038 &  Mercier Philip Cunningham was born in Centralia, Wash., on April 16, 1919. & (Mercier Philip Cunningham, was born in, Centralia) $\rightarrow$ (Merce Cunningham, was born in, Centralia); (Mercier Philip Cunningham, in, Wash.) $\rightarrow$ (Merce Cunningham, per:stateorprovince\_of\_birth, Wash.); (Mercier Philip Cunningham, in, April) $\rightarrow$ (Merce Cunningham, per:date\_of\_birth, 1919-04-16)\\ \hline
SF13\_ENG\_038 &  Cunningham's survivors include a brother, Jack Cunningham of Centralia. & (Cunningham'S Survivors, ,, Jack Cunningham) $\rightarrow$ (Merce Cunningham, per:siblings, Jack Cunningham)\\ \hline
SF13\_ENG\_041 & By the time Hewitt was 6, his family was living in New Rochelle, N.Y.  & (Hewitt, in, New Rochelle) $\rightarrow$ (Don Hewitt, per:cities\_of\_residence, New Rochelle)\\ \hline
SF13\_ENG\_041 &  He is survived by his third wife, former television news correspondent Marilyn Berger; his sons, Steven and Jeffrey; his daughter, Lisa Cassara; his stepdaughter, Jilian Childers Hewitt, whom Hewitt adopted; and three grandchildren. & (Hewitt, ,, Jilian Childers Hewitt) $\rightarrow$ (Don Hewitt, per:children, Jilian Childers Hewitt)\\ \hline
SF13\_ENG\_044 &  Dunne was born in 1925 in Hartford, Connecticut, to a wealthy Roman Catholic family and grew up in some of the same social circles as the Kennedys. & (Dunne, was born in 1925 in, Connecticut) $\rightarrow$ (Dominick Dunne, per:stateorprovince\_of\_birth, Connecticut)\\ \hline
SF13\_ENG\_044 &  Dunne was part of a famous family that also included his brother, novelist and screenwriter John Gregory Dunne; his brother's wife, author Joan Didion; and his son, Griffin. & (His Brother, ,, Novelist) $\rightarrow$ (His brother, per:title, Novelist)\\ \hline
SF13\_ENG\_044 &  Dunne and his wife, Ellen Griffin Dunne, known as Lenny, were married in 1954. & (Dunne, and, Ellen Griffin Dunne) $\rightarrow$ (Dominick Dunne, per:spouse, Ellen Griffin Dunne)\\ \hline
SF13\_ENG\_047 &  The women were accompanied by Reyna Luisa Tamayo, the mother of political prisoner Orlando Zapata, who died at age 42 in a hunger strike February 23 to protest prison conditions. & (Political Prisoner Orlando Zapata, ,, Reyna Luisa Tamayo) $\rightarrow$ (Orlando Zapata, per:children, Reyna Luisa Tamayo)\\ \hline
SF13\_ENG\_061 &  InterContinental Hotels Group, owners of Holiday Inn Worldwide, has been ordered by a court to pay \$25 million in damages to a franchisee for fraud. & (Intercontinental Hotels Group, ,, Holiday Inn Worldwide) $\rightarrow$ (InterContinental Hotels Group, org:parents, Holiday Inn Worldwide)\\ \hline
SF13\_ENG\_079 &  Water and its links to development, peace and conflict were key words in the annual sessions, Anders Berntell, executive director of Stockholm International Water Institute (SIWI), said in his opening address. & (Stockholm International, director, Anders Berntell) $\rightarrow$ (Stockholm International Water Institute, per:top\_members\_or\_employees, Anders Berntell); (Stockholm International, , executive director, Anders Berntell) $\rightarrow$ (Stockholm International Water Institute, per:top\_members\_or\_employees, Anders Berntell)\\ \hline
SF13\_ENG\_090 &  ECO member countries include Afghanistan, Azerbaijan, Iran, Kazakhstan, Kyrgyzstan, Pakistan, Tajikistan, Turkey, Turkmenistan and Uzbekistan. & (Eco Member Countries, ,, Azerbaijan) $\rightarrow$ (Economic Cooperation Organization, org:members, Azerbaijan)\\ \hline
SF13\_ENG\_096 &  A phone message left Sunday at Freedom's Irvine, California, headquarters was not immediately returned. & (Freedom'S Irvine, ,, California)$\rightarrow$ (Freedom Communications, org:stateorprovince\_of\_headquarters, California)\\ \hline
SF13\_ENG\_097 &  STX Finland is part of the international STX Europe Group, with shipyards in Brazil, Norway, France, Romania and Vietnam. & (Stx Finland, of, The International Stx Europe Group)$\rightarrow$ (STX Finland, org:subsidaries, The International Stx Europe Group)\\
