# Supplementary material for: IELM: An Open Information Extraction Benchmark for Pre-Trained Language Models
Source: arXiv:2210.14128 source file (2022-10-25)
Supplement: Supplementary file 6 [file unmapped_gpt2xl_wikidata.tex]

Douglas\_Bader & He left St Edward's in early 1928, aged 18. & (He, left, St Edward) $\rightarrow$ (douglas\_bader.Q348780, left, st\_edward's\_school,\_oxford.Q128260)\\ \hline
Douglas\_Bader & Group Captain Sir Douglas Robert Steuart Bader, was a Royal Air Force flying ace during the Second World War. & (Douglas Bader  Group Captain Sir Douglas Robert Steuart Bader, was, A Royal Air Force Flying Ace) $\rightarrow$ (douglas\_bader.Q348780, was, flying\_ace.Q222982)\\ \hline
Douglas\_Bader & On 2 July 1941 he was awarded the bar to his DSO. & (He, was awarded the bar to, his DSO) $\rightarrow$ (douglas\_bader.Q348780, was awarded the bar to, distinguished\_service\_order.Q615838) \\ \hline
Helen\_Storrow & His father, also named James Jackson Storrow, was a prominent attorney, whose clients included Alexander Graham Bell and the government of Venezuela; his mother, Ann Maria Perry, was the grandchild of naval hero Commodore Oliver Hazard Perry, and a distant cousin of President Thomas Jefferson. & (His Father, was, A Prominent Attorney) $\rightarrow$ (His Father, occupation.P106, lawyer.Q40348)\\ \hline
Helen\_Storrow & Helen Osborne Storrow was a prominent American philanthropist, early Girl Scout leader, and chair of the World Committee of the World Association of Girl Guides and Girl Scouts          for eight years. & (Helen Osborne Storrow, was, A Prominent American Philanthropist) $\rightarrow$ (helen\_storrow.Q5703224, was, united\_states.Q30)\\ \hline
Jacob\_Van\_Ruisdael & Ruisdael lived and worked in Amsterdam for the rest of his life. & (Ruisdael, lived, Amsterdam) $\rightarrow$ (jacob\_van\_ruisdael.Q213612, lived, amsterdam.Q727); (Ruisdael, lived and worked in, Amsterdam) $\rightarrow$ (jacob\_van\_ruisdael.Q213612, lived and worked in, amsterdam.Q727)\\ \hline
Liaquat\_Ali\_Khan & Liaquat Ali Khan was educated at the Aligarh Muslim University in India, and then at Oxford University in the United Kingdom. & (Liaquat Ali Khan, was educated at, The Aligarh Muslim University) $\rightarrow$ (liaquat\_ali\_khan.Q295713, was educated at, aligarh\_muslim\_university.Q196544)\\ \hline
Liaquat\_Ali\_Khan & After the death of his father in 1919, Ali Khan, with British Government awarding the grants and scholarship, went to England, attending Oxford University's Exeter College to pursue his higher education. & (His Higher Education, pursue, Oxford University'S Exeter College) $\rightarrow$ (liaquat\_ali\_khan.Q295713, pursue, university\_of\_oxford.Q34433)\\ \hline
Liaquat\_Ali\_Khan & In 1940, Khan was made the deputy leader of the Muslim League Parliamentary party. & (Khan, was made the deputy leader of, The Muslim League Parliamentary Party) $\rightarrow$ (liaquat\_ali\_khan.Q295713, deputy leader, all-india\_muslim\_league.Q223898)\\ \hline
Pauline\_Baynes &   When Baynes's father retired, he left India and returned to England, settling with Baynes's mother in a house close to Baynes's own near Farnham in southwest Surrey. & (He, left, India) $\rightarrow$ (pauline\_baynes.Q101951, left, india.Q668)\\ \hline
Pauline\_Baynes &   Baynes began her education at a convent school. & (Her Education, at, A Convent School) $\rightarrow$ (pauline\_baynes.Q101951, at, catholic\_school.Q1138671)\\ \hline
Pauline\_Baynes & Her most vivid recollection of their New Year's Eve lunch at Magdalen College was of his gleefully picking nuts out of a bowl of Brussels sprouts. & (Their New Year'S Eve Lunch, at, Magdalen College) $\rightarrow$ (pauline\_baynes.Q101951, at, magdalen\_college,\_oxford.Q81162)\\ \hline
Pauline\_Baynes & She was not a diligent student, frittering away her time on \"coffee and parties\", and she left the Slade without a qualification, But she did achieve the distinction, one shared with her sister, of exhibiting at the Royal Academy of Arts in 1939. In 1940, a year into World War II, both Baynes sisters joined the Women's Voluntary Service. & (She, without a qualification, The Slade) $\rightarrow$ (pauline\_baynes.Q101951, without a qualification, slade\_school\_of\_fine\_art.Q1399299)\\ \hline
Thor\_Heyerdahl & His theories rarely won any scientific acceptance, whereas Heyerdahl himself rejected all scientific criticism and concentrated on publishing his theories in popular books aimed at the general public. & (His Theories, at, The General Public) $\rightarrow$ (thor\_heyerdahl.Q133622, at, general\_public)\\ \hline
Thor\_Heyerdahl & He was an atheist. & (He, was, An Atheist) $\rightarrow$ (thor\_heyerdahl.Q133622, was, An Atheist)\\ \hline
Neville\_Southall &   As a teenager, Southall had unsuccessful trials at Wrexham, Crewe Alexandra and Bolton Wanderers. & (Southall, at, Wrexham) $\rightarrow$ (neville\_southall.Q436650, at, wrexham\_a.f.c..Q18529); (Southall, at, Crewe Alexandra) $\rightarrow$ (neville\_southall.Q436650, at, crewe\_alexandra\_f.c..Q19587)\\ \hline
John\_Maynard\_Keynes & John Maynard Keynes, 1st Baron Keynes, was a British economist, whose ideas fundamentally changed the theory and practice of macroeconomics and the economic policies of governments. & (John Maynard Keynes, was, A British Economist) $\rightarrow$ (john\_maynard\_keynes.Q9317, was, united\_kingdom.Q145)\\ \hline
John\_Maynard\_Keynes &   In January 1889 at the age of five and a half, Keynes started at the kindergarten of the Perse School for Girls for five mornings a week. & (Keynes, at, The Perse School) $\rightarrow$ (john\_maynard\_keynes.Q9317, at, the\_perse\_school.Q7756751)\\ \hline
John\_Maynard\_Keynes & In January 1892, at eight and a half, he started as a day pupil at St Faith's preparatory school. & (He, at, St Faith'S Preparatory School) $\rightarrow$ (john\_maynard\_keynes.Q9317, at, st\_faith's\_school.Q7593056)\\ \hline
John\_Maynard\_Keynes & Keynes was a lifelong member of the Liberal Party, which until the 1920s had been one of the two main political parties in the United Kingdom, and as late as 1916 had often been the dominant power in government. & (Keynes, was a lifelong member of, The liberal party) $\rightarrow$ (john\_maynard\_keynes.Q9317, was a lifelong member of, liberal\_party\_(uk).Q622441) \\ \hline
Ernst\_Haeckel &   Haeckel was awarded the title of Excellency by Kaiser Wilhelm II in 1907 and the Linnean Society of London's prestigious Darwin-Wallace Medal in 1908. & (Haeckel, was awarded the, Excellency) $\rightarrow$ (ernst\_haeckel.Q48246, award\_received.P166, Excellency)\\ \hline
Ernst\_Haeckel & He was also a pacifist until the First World War, when he wrote propaganda in favor of the war. & (He, was, A Pacifist) $\rightarrow$ (ernst\_haeckel.Q48246, was, A Pacifist)\\ \hline
Ernst\_Haeckel & He was also a social Darwinist who believed that "survival of the fittest" was a natural law, and that struggle led to improvement of the race. & (He, was, A Social Darwinist) $\rightarrow$ (ernst\_haeckel.Q48246, was, A Social Darwinist)\\ \hline
Ernst\_Haeckel & Ernst Haeckel was born on 16 February 1834, in Potsdam. & (Haeckel, was born on 17 February 1834, in, Potsdam) $\rightarrow$ (ernst\_haeckel.Q48246, was born on 17 February 1834, in, potsdam.Q1711) \\
