# Supplementary material for: IELM: An Open Information Extraction Benchmark for Pre-Trained Language Models
Source: arXiv:2210.14128 source file (2022-10-25)
Supplement: Supplementary file 7 [file appendix_old.tex]

% \maketitle
% ~
% \newpage
% ~
\newpage

\section{Additional Details}
\label{sec:adddetails}

\subsection{Method Details}
\label{sec:implement}

\paragraph{Evaluation Details} To evaluate the triples, we first use the knowledge calibration module to run over the corresponding documents to generate the triples. For out-of-domain TAC KBP, we link to the oracle annotation of the entities or spans in the TAC KBP corpus. For in-domain Wikidata, the entity linking method described in Sec.~\ref{sec:evalmethod} is first leveraged to link entities in the triples to Wikipedia anchors. We build an enhanced mention-to-entity dictionary based on ~\citep{spitkovsky2012cross}. In particular, we add new Wikipedia anchors to the dictionary which results in 26 million entries compared to 21 million entries in ~\citep{spitkovsky2012cross}. Then a Wikipedia anchor to the Wikidata item dictionary is constructed and used to further link the entities to Wikidata. If the head or tail is a pronoun, we further use neuralcoref~\footnote{\tiny\url{https://github.com/huggingface/neuralcoref}} for coreference resolution. We use GloVe~\citep{pennington2014glove} embedding for disambiguation. The relation mapping is constructed offline for Wikidata using the method in Sec.~\ref{sec:evalmethod}. Besides the automatic relation mapping method proposed in ~\citep{angeli2015leveraging}, we manually check whether the top relation phrases are true as described in Sec.~\ref{sec:evalmethod}. For relation mapping, we randomly sampled a hold-out dataset including 2,000 documents from English Wikipedia for the relation mapping construction on Wikidata. For oracle facts in Wikidata, we only preserve those facts describing relations between entities that could be linked to corresponding Wikipedia anchors. We rule out facts of attributes about entities and facts of auxiliary relations (such as \textit{topic's main category.P901}) and finally result in 27,368,562 oracle facts.

\paragraph{Implementation Details} For Wikidata, we randomly split the English Wikipedia data into 20 partitions, and map the data partitions to 20 distributed servers to run. Each server is configured with four Tesla K80 12Gs. We set the max sequence length to 256, and batch size as 32 for BERT$_{\rm LARGE}$ and 4 for GPT-2$_{\rm XL}$. We use implementations of pre-trained LMs in the Transformers package~\footnote{\tiny\url{https://github.com/huggingface/transformers}}. We use spaCy sentencizer~\footnote{{\tiny\url{https://spacy.io/api/sentencizer}}} to segment the documents into sentences. BERT$_{\rm LARGE}$ takes approximately 48 hours, and GPT-2$_{\rm XL}$ costs around 96 hours. The resulting triples of knowledge calibration from the 20 servers are then reduced to a data server, where a MongoDB database is maintained to store the oracle Wikidata and entity linking results to enable the efficient evaluation stage. The batch sizes of BERT$_{\rm BASE}$, GPT-2, GPT-2$_{\rm MEDIUM}$, GPT-2$_{\rm LARGE}$ are 64, 32, 16, 8 respectively.

\paragraph{Parameter Settings} The parameter settings are shared across in-domain Wikidata and out-of-domain TAC KBP. All the choices are based on the parameter study in Sec.~\ref{sec:para}. The beam size of Algorithm~\ref{alg:beamsearch} is set to 6. The attention score threshold is set to 0.005, and the number of distinct head-tail pairs is set to 10. To generate the attention weight matrix $\mathbf{A}_s$ of a sentence, we reduce the weights of every attention head in the last layer of pre-trained LMs using the mean operator.  

\paragraph{Predicate Extraction as Beam Search} The inputs of the search algorithm are a head-tail pair $(h,t)$, a sentence $s$, an attention matrix $\mathbf{A}_s$ of $s$. Both $h$ and $t$ are identified by the noun chunk in $s$. $\mathbf{A}_s$ is the attention matrix associated with $s$ from the forward pass of LM without fine-tuning. The search gets started by adding the head $h$ as the initial candidate in the beam. While there are still new candidates waiting to be yielded, the search continues, and the top $k$ candidates sorted by the attention scores are maintained in the beam.
The details of the proposed beam search are in Algorithm~\ref{alg:beamsearch}. In practice, we implement an action manager $\mathcal{O}$ to decide which action to take at each step. Given a candidate $c$ in the beam, $\mathcal{O}(c) = \texttu{start}$ always happens at the beginning of the search. If $c$ has not reached the tail $t$ yet, $\mathcal{O}(c) = \mathbf{\texttu{yield}}$. Otherwise, $\mathcal{O}(c) = \texttu{stop}$.

\begin{algorithm}[tb]
\small
% \vspace{-0.05in}
\caption{\label{alg:beamsearch}{Beam search with attention scores.}}
\begin{algorithmic}[1]
\Require{Head-tail pair $(h,t)$, sentence $s$, attention matrix $\mathbf{A_s}$, action manager $\mathcal{O}=\{\texttu{start}, \texttu{yield}, \texttu{stop}\}$, beam size $k$}
\Ensure{Triples $\mathbb{T}_{(h,t)}$}
\State $\mathbb{T}_{(h,t)} \leftarrow \{\texttu{start}(h)\}$ 
\Comment{{\em Start} by adding the head as a candidate in the beam}
\While{$\exists c \in \mathbb{T}_{(h,t)} [\mathcal{O}(c) = \texttu{yield}]$} 
\State $\widetilde{\mathbb{T}}_{(h,t)} \leftarrow \emptyset$ 
\Comment{Initialize a new beam}
\ForAll{$c \in \mathbb{T}_{(h,t)}$}
\If{$\mathcal{O}(c) = \texttu{yield}$} 
\State $\widetilde{\mathbb{T}}_{(h,t)} \leftarrow  \widetilde{\mathbb{T}}_{(h,t)} \cup \{\texttu{yield}(c,s,\mathbf{A}_s)\}$ \Comment{{\em Yield} a new candidate if not reached the tail}
\Else
\State $\widetilde{\mathbb{T}}_{(h,t)} \leftarrow  \widetilde{\mathbb{T}}_{(h,t)} \cup \{\texttu{stop}(c,t)\}$ \Comment{{\em Stop} then produce a valid fact if reached the tail}
\EndIf
\EndFor
\State $\mathbb{T}_{(h,t)} \leftarrow {\rm TOP}(k, \widetilde{\mathbb{T}}_{(h,t)})$ \Comment{Maintain $k$-best candidates in the beam}
\EndWhile
\State \Return $\mathbb{T}_{(h,t)}$
\end{algorithmic}
\end{algorithm}

\subsection{Comparison Methods}
\xiao{add}
We compare with the following OIE systems. (\expandafter{\romannumeral1}) Neural network (NN) based OIE:
\begin{itemize}[leftmargin=*]
    \item SenseOIE~\citep{roy2019supervising},  
    \item SpanOIE~\citep{zhan2020span}\footnote{\tiny\url{https://github.com/zhanjunlang/Span_OIE}}, 
    \item RnnOIE~\citep{stanovsky2018supervised}\footnote{\tiny\url{https://github.com/gabrielStanovsky/supervised-oie}} is one of the state-of-the-art OIE systems. It uses LSTM to model the OIE problem as a sequence tagging problem, and is trained on a large-scale OIE training set.
    \item NeuralOIE~\citep{cui2018neural}\footnote{\tiny We use the BERT implementation (CopyAttn+BERT) available at \url{https://github.com/dair-iitd/imojie}},
    \item IMoJIE~\citep{kolluru2020imojie}\footnote{\tiny\url{https://github.com/dair-iitd/imojie}} is a sequence generation OIE model that uses BERT at encoding time.
    \item Multi$^2$OIE~\citep{ro2020multi}\footnote{\tiny\url{https://github.com/youngbin-ro/Multi2OIE}} models OIE as a sequence-labeling problem that combines BERT with multi-head attention blocks.
    \item OpenIE6~\citep{kolluru2020openie6}\footnote{\tiny\url{https://github.com/dair-iitd/openie6}} is one of the state-of-the-art OIE systems. It treats OIE as a 2-D grid labeling task, and trains a BERT like architecture for the task.
\end{itemize}

(\expandafter{\romannumeral2}) Linguistic pattern based OIE: 
\begin{itemize}[leftmargin=*]
    \item MinIE~\citep{gashteovski2017minie}\footnote{\tiny\url{https://github.com/uma-pi1/minie}},                 
    \item ClausIE~\citep{del2013clausie}\footnote{\tiny\url{https://www.mpi-inf.mpg.de/departments/databases-and-information-systems/research/ambiverse-nlu/clausie}}, 
    \item OLLIE~\citep{schmitz2012open}\footnote{\tiny\url{https://github.com/knowitall/ollie}},
    \item PropS~\citep{stanovsky2016getting}\footnote{\tiny\url{https://github.com/gabrielStanovsky/props}},
    \item OpenIE4~\citep{christensen2011analysis}\footnote{\tiny\url{https://github.com/allenai/openie-standalone}},
    \item OpenIE5~\citep{saha2017bootstrapping,saha2018open}\footnote{\label{ft:openie51}\tiny\url{https://github.com/dair-iitd/OpenIE-standalone}} is one of the state-of-the-art OIE systems, which is the successor to OLLIE, and it improves extractions from noun relations, numerical sentences, and conjunctive sentences depending on the linguistic patterns. 
    \item Stanford OpenIE~\citep{angeli2015leveraging} leverages POS tag and dependency parser, and generates self-contained clauses from long sentences to extract the triples. 
\end{itemize}
Note that all the NN OIE systems are supervised.

\subsection{Additional Analysis of Parameter Study}
\label{sec:morepara}

\paragraph{Effects of Beam Size} Figure~\ref{fig:para}(a) illustrates the effects of various beam sizes in Algorithm~\ref{alg:beamsearch}. We find that in general, the larger the beam size is, the better F1 the setting achieves. This is because our method is able to reserve more potentially correct facts when more candidates are allowed in the knowledge calibration. However, F1 improvement gradually becomes subtle, while the computation costs increase more significantly. For efficiency, we do not explore larger beam sizes. We set the beam size as 6.

\paragraph{Effects of Search Constraints} Figure~\ref{fig:para}(b) compares the effect of different thresholds of the total score. We set the threshold as 0.005 since it achieves the best result. Note that the summed attention score is normalized by the length of the fact to penalize the cumbersome facts. The threshold is effective, which is mainly because of the knowledge contained in the self-attention matrix. The score in the attention matrix is representing the chance of the facts to be the true facts based on the stored knowledge. Figure~\ref{fig:para}(c) shows the impact of the number of distinct head-tail pairs in identifying common relations. The best result is achieved when it equals 10. This shows that while our method mostly identifies frequent relations, it is also able to capture some rare relations.

\paragraph{Effects of Attention Weights} Figure~\ref{fig:para}(d) shows the comparison between attention weights of the last layer and the mean of all layers. The attention weights of the last layer perform better. This is due to the attention weights in lower layers are low-level linguistic knowledge according to \citep{clark2019does,ramsauer2020hopfield}, which are less relevant to the factual knowledge. Figure~\ref{fig:para}(e) compares the impact of different attention reduction, i.e., mean, max, over the attention heads of the last layer. We find the ``mean'' performs better. The reason is that the token often intensively attends to several specific tokens in the sequence~\citep{michel2019sixteen}, and the ``mean'' operator is less sensitive to such information.


\section{Samples from TAC KBP-OIE}

We randomly sample 100 documents from TAC KBP corpus, then randomly sample sentences from those documents. 
The uncurated triples and the corresponding mapped facts of the sampled sentences based on our best methods
BERT$_{\rm LARGE}$ and GPT-2$_{\rm XL}$ are shown in Figure~\ref{fig:kbpmapbert} and Figure~\ref{fig:kbpmapgpt} respectively.
We also randomly sample several sentences in which BERT$_{\rm LARGE}$ differs from GPT-2$_{\rm XL}$ in the resulting facts for comparison, which is illustrated in Figure~\ref{fig:kbpmapbertgpt}.
In each table, ``{\bf ID}'' represents the document ID of a sampled sentence in TAC KBP corpus. ``{\bf Sentence}'' indicates the sampled sentence. ``{\bf Triples to mapped facts}'' column contains the triples (on the left side of ``$\rightarrow$'') and their corresponding mapped facts (on the right side of ``$\rightarrow$'').

\section{Samples from Wikidata-OIE}
\label{seca:wiki}

Similar to TAC KBP, we randomly sample 100 documents from the Wikidata corpus (i.e., English Wikipedia), then randomly sample sentences from those documents. 
The uncurated triples and the corresponding mapped facts of the sampled sentences based on our best method BERT$_{\rm LARGE}$ are shown in Figure~\ref{fig:wikimapbert}.
% We also randomly sample several sentences in which BERT$_{\rm LARGE}$ differs from GPT-2$_{\rm XL}$ in the resulting facts for comparison, which is illustrated in Figure~\ref{fig:wikimapbertgpt}.
In each table, ``{\bf ID}'' represents the Wikipedia page's title of a sampled sentence. ``{\bf Sentence}'' indicates the sampled sentence. ``{\bf Triples to mapped facts}'' column contains the triples (on the left side of ``$\rightarrow$'') and their corresponding mapped facts (on the right side of ``$\rightarrow$'').

%  and GPT-2$_{\rm XL}$  and Figure~\ref{fig:wikimapgpt} respectively

\begin{figure*}
\begin{center}
\tiny
\resizebox{0.85\linewidth}{!}
  {
\begin{tabular}{l p{11cm} p{11cm}}
\toprule
{\bf ID} & {\bf Sentence} & {\bf Triples to mapped facts} \\ \hline
\input{appendices_table/mapped_bertlarge_kbp}
\bottomrule
\end{tabular}
}
\end{center}
\vspace{-0.1in}
\caption{{\small BERT$_{\rm LARGE}$ on TAC KBP.}} \label{fig:kbpmapbert}
\end{figure*}


\begin{figure*}
\begin{center}
\tiny
\resizebox{0.81\linewidth}{!}
  {
\begin{tabular}{l p{11cm} p{11cm}}
\toprule
{\bf ID} & {\bf Sentence} & {\bf Triples to mapped facts} \\ \hline
\input{appendices_table/mapped_gpt2xl_kbp}
\bottomrule
\end{tabular}
}
\end{center}
\caption{{\small GPT-2$_{\rm XL}$ on TAC KBP.}} \label{fig:kbpmapgpt}
\end{figure*}


\begin{figure*}
\begin{center}
\tiny
\resizebox{0.85\linewidth}{!}
  {
\begin{tabular}{l p{7cm} p{7cm} p{7cm}}
\toprule
\multirow{2}{*}{\bf ID} & \multirow{2}{*}{\bf Sentence} & \multicolumn{2}{c}{\bf Triples to mapped facts} \\
& & {\bf BERT$_{\rm LARGE}$} & {\bf GPT-2$_{\rm XL}$} \\ \hline
\input{appendices_table/mapped_compare_kbp}
\bottomrule
\end{tabular}
}
\end{center}
\caption{{\small BERT$_{\rm LARGE}$ vs. GPT-2$_{\rm XL}$ on TAC KBP.}} \label{fig:kbpmapbertgpt}
\end{figure*}





\begin{figure*}
\begin{center}
\tiny
\resizebox{0.81\linewidth}{!}
  {
\begin{tabular}{l p{10cm} p{10cm}}
\toprule
{\bf ID} & {\bf Sentence} & {\bf Triples to mapped facts} \\ \hline
\input{appendices_table/mapped_bertlarge_wikidata}
\bottomrule
\end{tabular}
}
\end{center}
\caption{{\small BERT$_{\rm LARGE}$ on Wikidata.}} \label{fig:wikimapbert}
\end{figure*}


% \begin{figure*}
% \begin{center}
% \tiny
% \resizebox{0.85\linewidth}{!}
%   {
% \begin{tabular}{l p{10cm} p{10cm}}
% \toprule
% {\bf ID} & {\bf Sentence} & {\bf Triples to mapped facts} \\ \hline
% \input{appendices_table/mapped_gpt2xl_wikidata}
% \bottomrule
% \end{tabular}
% }
% \end{center}
% \caption{{\small GPT-2$_{\rm XL}$ on Wikidata.}} \label{fig:wikimapgpt}
% \end{figure*}


% \begin{figure*}
% \begin{center}
% \tiny
% \resizebox{0.85\linewidth}{!}
%   {
% \begin{tabular}{l p{7cm} p{7cm} p{7cm}}
% \toprule
% \multirow{2}{*}{\bf ID} & \multirow{2}{*}{\bf Sentence} & \multicolumn{2}{c}{\bf Triples to mapped facts} \\
% & & {\bf BERT$_{\rm LARGE}$} & {\bf GPT-2$_{\rm XL}$} \\ \hline
% \input{appendices_table/mapped_compare_wikidata}
% \bottomrule
% \end{tabular}
% }
% \end{center}
% \caption{{\small BERT$_{\rm LARGE}$ vs. GPT-2$_{\rm XL}$ on Wikidata.}} \label{fig:wikimapbertgpt}
% \end{figure*}
